# Supplementary material for: Efficient Learning of Interpretable Classification Rules
Source: arXiv:2205.06936 source file (2022-08-30)
Supplement: Supplementary file 1 [file explanation.tex]

\subsection{Illustration of Incremental Learning}
%Step by step rule formulation for an example
	\label{sec:example}
	We illustrate  an interpretable rule generated by $ \IMLI $ with step by step formulation over partitions on iris dataset\footnote{\url{https://archive.ics.uci.edu/ml/datasets/iris}}. Iris dataset has four attributes: sepal length, sepal width, petal length, and petal width. All feature values are scaled in centimeter. Iris dataset has three classes: Iris Setosa, Iris Versicolour, and Iris Virginica. We consider the binary problem of classifying Iris Versicolour  from the other two species: Setosa and Verginica. Here we consider that $ \R $ is a single clause  DNF rule and learned over four partitions (e.g. $ \R_1, \dots, \R_4 $). The final rule $ \R $  is equivalent to $ \R_4 $. 
	
%	At first, we show $ \R_\MLIC $, the interpretable rule generated by $ \MLIC $ on the same parameter setting.
%	\begin{equation*}
%	\begin{split}
%	&\R_\MLIC:=\text{sepal width} \le 3.2 \,\wedge \, \text{petal length} \le 5.0 \,\wedge \, \\ 
%	& \qquad \qquad \quad\text{petal length} > 1.7\,\wedge \, \text{petal width} \le 1.5
%	\end{split}
%	\end{equation*}

\begin{equation*}
\begin{split}
&\R_1:=\text{petal length} \le 5.32 \,\wedge \, \text{petal length} > 1.7 \,\wedge \, \\
&\qquad\;\;\;\text{petal width} \le 1.8\\
&\R_2:=\text{sepal width} \le 3.1 \,\wedge \, \text{petal length} \le 5.32 \,\wedge \,\\ &\qquad\;\;\;\text{petal length} > 1.7 \,\wedge \, \text{petal width} \le 1.5\\
&\R_3:=\text{sepal width} \le 3.1 \,\wedge \, \text{petal length} \le 5.0 \,\wedge \,\\ &\qquad\;\;\;\text{petal length} > 1.7 \,\wedge \, \text{petal width} \le 1.5\\
& \R:=\text{sepal width} \le 3.1 \,\wedge \, \text{petal length} \le 5.0 \,\wedge \,\\ &\qquad\;\;\;\;\;\;\;\text{petal length} > 1.7 \,\wedge \, \text{petal width} \le 1.8
\end{split}
\end{equation*}
$ \R $ can be interpreted as: 
	a sample which satisfies all of the four constraints is predicted as Iris Versicolour. Here the  rule size $ | \R|=4 $. Specifically, $ \R_1 $ is learned on the first partition of training data. $ \R_2 $ learns two literals ($ 2^{nd} $ and $ 3^{rd} $) which also appear in $ \R_1 $, introduces two new literals ($ 1^{st} $ and $ 4^{th} $) while learning on the second training partition, and falsifies a previously learned literal  from $ \R_1 $ (i.e., $ (\text{petal width} \le 1.8 $). 
	
	Since the dataset contains continuous valued features, $ \IMLI $ removes redundant literals at each step of learning by applying  Algorithm \ref{alg:imli-RRL}. For example, we show the  generated rule $ \R_3' $  for the $ 3^{rd} $ partition if we do not apply Algorithm \ref{alg:imli-RRL}.

%	 ($ 1^{st} $, and $ 2^{nd} $ literal). $ \R_2 $ does not contain the $ 3^{rd} $ literal of $ \R_1 $ because $ \IMLI $ learns $ \sigma_2(\text{petal width} \le 1.8)=0 $. Note that the $ 1^{st} $ literal of $ \R_2 $ is not in $ \R_1 $ but appears in $ \R_2 $.  We notice that initial learned rule is shorter in length (e.g., $ |\R_1|=3 $), however, as we learn rule for more training batches, rule size increases (e.g., $ |\R_2|=|\R_3|=|\R_4|=4 $). 
%
%\begin{equation*}
%	\begin{split}
%	&\R_1':=\text{petal length} \le 5.32 \,\wedge\, \text{petal length} > 1.7 \,\wedge\,\\
%	 &\qquad\;\;\;\text{petal width} \le 1.8\\
%	&\R_2':=\text{sepal width} \le 3.1 \,\wedge\, \text{petal length} \le 5.32 \,\wedge\,\\
%	 &\qquad\;\;\;\text{petal length} > 1.7 \,\wedge\, \text{petal width} \le 1.5 \,\wedge\,\\
%	  &\qquad\;\;\;\underline{\text{petal width} \le 1.8}\\
%	&\R_3':=\text{sepal width} \le 3.1 \,\wedge\, \text{petal length} \le 5.0 \,\wedge\, \\
%	&\qquad\;\;\;\underline{\text{petal length} \le 5.32} \,\wedge\, \text{petal length} > 1.7 \,\wedge\, \\
%	&\qquad\;\;\;\text{petal width} \le 1.5 \,\wedge\, \underline{\text{petal width} \le 1.8}\\
%	&\R_4':=\text{sepal width} \le 3.1 \,\wedge\, \text{petal length} \le 5.0 \,\wedge\, \\
%	&\qquad\;\;\;\underline{\text{petal length} \le 5.32} \,\wedge\, \text{petal length} > 1.7 \,\wedge\, \\
%	&\qquad\;\;\;\text{petal width} \le 1.8
%	\end{split}
%\end{equation*}
%	

\begin{equation*}
\begin{split}
&\R_3':=\text{sepal width} \le 3.1 \,\wedge\, \text{petal length} \le 5.0 \,\wedge\, \\
&\qquad\;\;\;\underline{\text{petal length} \le 5.32} \,\wedge\, \text{petal length} > 1.7 \,\wedge\, \\
&\qquad\;\;\;\text{petal width} \le 1.5 \,\wedge\, \underline{\text{petal width} \le 1.8}\\
\end{split}
\end{equation*}

	The underline marked literals are redundant, hence removed in $\R_3 $.
