# Supplementary material for: Efficient Learning of Interpretable Classification Rules
Source: arXiv:2205.06936 source file (2022-08-30)
Supplement: Supplementary file 2 [file improvement.tex]

\section{Extra... previous}
\section{Improving the baseline}

\begin{comment}
		\begin{itemize}
		\item The number of clauses in the MaxSAT query is $ \mathcal{O}(k \cdot m \cdot n) $. We want to reduce the query size by addressing all the dependent parameters. 
		\item Learning single clause rule is easier than learning a multi-clause rule. 
		\item 
		\item We adopt mini-batch learning where we consider a reduced number of samples generated i.i.d. from the original training data. Since want to learn the value of discrete decision variables and the cost function is non-differentiable, it is tricky (may be impossible) to learn the optimum value because no convergence guarantee is available for discrete problem.  We propose a solving technique where we modify the value of a decision variable only if it tries to  optimize the cost function.
		
		\end{itemize}
		\begin{theorem}
		If a  training  sample   is predicted false by clause $ C_l $ in the $ l $-th iteration, the sample is also be predicted false by a CNF formula including clause $ C $. 
		Therefore,  the sample  can be removed from the training set while learning $ C_{l+1} $.
		\end{theorem}
		
\end{comment}

In this section, we discuss how to improve the  proposed MaxSAT formulation in Section~\ref{sec:encoding}. In particular, we discuss how to reduce both the  number of variables and the number of clauses in the formulation. The complexity of the MaxSAT query depends on three factors: the number of binary features $ m $,  the number of clauses  $ k $ in the desired rule, and the size of the  training set $ n $.    Therefore, we propose to (i)  rank features based on their contribution to the correctness in prediction and consider only more important features in Section~\ref{sec:feature_elimination}, (ii)  learn a single clause rule iteratively on a reduced training set in Section~\ref{sec:iterative_learning}, and (iii) learn rules in  a novel incremental  mini-batch approach tailored for  the discrete optimization problem in Section~\ref{sec:incremental_learning}.  Finally  in Section~\ref{sec:all_hypotheses}, we  discuss an improved formulation that takes benefit of all three proposed hypotheses.

\subsection{Feature Ranking}
\label{sec:feature_elimination}

	All features in the training dataset do not contribute similarly in the prediction and thus do not appear in rule $ \Rule $. In the following, we  rank features based on their individual contribution to the accuracy of $ \Rule $ and propose to  formulate the MaxSAT query with higher ranked features. \red{cite dmitry and show difference}
	
%	We rank features with the assumption that $ \Rule $ is a single clause rule and empirically show that this assumption does not affect the prediction accuracy of multi-clause rules.
	We rank features considering both feature-value and  class label of samples in the training set. For the $ j $-th feature, we measure the number of  positive labeled samples having feature-value $ 1 $ (denoted as $ \mathsf{TP}_j $) and the number of  negative labeled samples having feature-value $ 1 $ (denoted as $ \mathsf{FP}_j $) in the training set $ (\mathbf{X}, \mathbf{y}) $.
	\[
	\begin{split}
		 &\mathsf{TP}_j= \sum_{i=1}^{|\mathbf{X}|} \mathds{1}_{y_i=1 \;\wedge\; \mathbf{X}_{i,j}=1}\\
		 &\mathsf{FP}_j= \sum_{i=1}^{|\mathbf{X}|} \mathds{1}_{y_i=0 \;\wedge\; \mathbf{X}_{i,j}=1}
	\end{split}
	\]

	 In order to rank  features based on their individual contribution  to the prediction accuracy, we use $ \mathsf{TP}_j -\mathsf{FP}_j $ as the ranking metric such that features with higher value of $ \mathsf{TP}_j -\mathsf{FP}_j $ have higher rank.  Avoiding notational clutter, we overload $ \mathsf{TP}_C $ and $ \mathsf{FP}_C $  on a  disjunction of features in the  clause $ C $ as follows.

	\[
	\begin{split}
	&\mathsf{TP}_C= \sum_{i=1}^{|\mathbf{X}|} \mathds{1}_{y_i=1 \;\wedge\; (\bigvee_{j|b_j \in C}\mathbf{X}_{i,j}=1)}\\
	&\mathsf{FP}_C= \sum_{i=1}^{|\mathbf{X}|} \mathds{1}_{y_i=0 \;\wedge\; (\bigvee_{j|b_j \in C}\mathbf{X}_{i,j}=1)}
	\end{split}
	\]
	
	Exact computation of $ \mathsf{TP}_C $ and $ \mathsf{FP}_C $ is computationally expensive because one would require to find the disjunction of features in $ C $ for all samples. However, it is easier to find their upper bound $ \mathsf{UB}(\cdot) $ and  lower bound $ \mathsf{LB}(\cdot) $. In particular,  $ \mathsf{UB}(\mathsf{TP}_C) = \sum_{j|b_j \in C} \mathsf{TP}_j $, $ \mathsf{LB}(\mathsf{TP}_C) = \max_{j|b_j \in C} \mathsf{TP}_j $,  $ \mathsf{UB}(\mathsf{FP}_C) = \sum_{j|b_j \in C} \mathsf{FP}_j $, and $ \mathsf{LB}(\mathsf{FP}_C) = \max_{j|b_j \in C} \mathsf{FP}_j $.

	In the following, we show the justification of using $ \mathsf{TP}_j -\mathsf{FP}_j $ as the ranking metric.

	\begin{theorem}
		\label{theorem:ub_of_acc}
		Let $ C $ and $ C' $ be two clauses  differing in  one  feature, namely feature $ j $ and feature $ j' $ respectively, and $ \mathsf{TP}_j - \mathsf{FP}_j > \mathsf{TP}_{j'} - \mathsf{FP}_{j'} $. Then 
		$ \mathsf{UB}(\mathsf{TP}_{C}-\mathsf{FP}_{C}) > \mathsf{UB}(\mathsf{TP}_{C'}-\mathsf{FP}_{C'})  $.
	\end{theorem}

%	\end{theorem}
	
	\begin{proof}
		\red{need to rewrite}
		\label{proof:ub_of_acc}
		\[
		\begin{split}
		& \sum_{b_i \in C} \mathsf{TP}_i \ge \mathsf{TP}_C \ge \max_{i:b_i \in C}  \mathsf{TP}_i\\
		& \sum_{b_i \in C} \mathsf{FP}_i \ge \mathsf{FP}_C \ge \max_{i:b_i \in C}  \mathsf{FP}_i\\
		\end{split}
		\]
		Therefore, 
		\[
			\mathsf{TP}_C-  \mathsf{FP}_C \le 	\sum_{b_i \in C} \mathsf{TP}_i - \max_{i:b_i \in C}  \mathsf{FP}_i
		\]

		Now
		\[
		\mathsf{TP}_{C_{(j)}} -  \mathsf{FP}_{C_{(j)}} \le 	\sum_{b_i \in C} \mathsf{TP}_i - \max_{i:b_i \in C}  \mathsf{FP}_i \le \sum_{b_i \in C \wedge i\ne j} \mathsf{TP}_i + \mathsf{TP}_j- \mathsf{FP}_j 
		\]
		Similarly,
		\[
		\mathsf{TP}_{C_{(j')}} -  \mathsf{FP}_{C_{(j')}} \le \sum_{b_i \in C \wedge i\ne j'} \mathsf{TP}_i + \mathsf{TP}_{j'}- \mathsf{FP}_{j'} 
		\]
		Since $ \mathsf{TP}_j - \mathsf{FP}_j > \mathsf{TP}_{j'} - \mathsf{FP}_{j'} $, we  deduce following conclusion regarding the upper bound.
		\[
		\mathsf{UB}(\mathsf{TP}_{C_{(j)}}-\mathsf{FP}_{C_{(j)}}) > \mathsf{UB}(\mathsf{TP}_{C_{(j')}}-\mathsf{FP}_{C_{(j')}})
		\]
			\end{proof}
	
	\subsection{Feature Elimination}
	
	We refer to the  accuracy of a clause in $ \Rule $ as proportional to the difference between true positive and false positive samples covered by the clause. While constructing the MaxSAT query, we can eliminate a feature that cannot increase the accuracy of the clause in which it may be included. The following theorem states when to eliminate feature $ j $ depending on the value of $ \mathsf{TP}_j - \mathsf{FP}_j $ in the training set.

	\begin{theorem}
		Consider two clauses $ C $ and $ C_{(\setminus j)} $ such that $ C_{(\setminus j)} $ has all features of $ C $ except feature $ j $. If  $ \mathsf{TP}_j - \mathsf{FP}_j < 0 $, then  $ \mathsf{UB}(\mathsf{TP}_{C}-\mathsf{FP}_{C}) < \mathsf{UB}(\mathsf{TP}_{C_{(\setminus j)}}-\mathsf{FP}_{C_{(\setminus j)}}) $, and feature $ j $ can be eliminated.
	\end{theorem}

%	\begin{theorem}
%		Let $ C_{(j)} $ and $ C_{(\setminus j)} $ 
%		If   $ \mathsf{TP}_j - \mathsf{FP}_j < 0 $ for the $ j $-th feature, removing this feature will increase the upper bound on accuracy of a clause in a CNF rule.
%	\end{theorem}

	\begin{proof}
		From Proof~\ref{proof:ub_of_acc}
		\[
		\begin{split}
				&\mathsf{TP}_C -  \mathsf{FP}_C \le \sum_{b_i \in C \wedge i\ne j} \mathsf{TP}_i + \mathsf{TP}_{j}- \mathsf{FP}_{j} \\
		&\mathsf{TP}_{C_{(\setminus j)} } -  \mathsf{FP}_{C_{(\setminus j)} } \le \sum_{b_i \in C_{(\setminus j)}} \mathsf{TP}_i 
		\end{split}
		\]
		 Since $  \sum_{b_i \in C \wedge i\ne j} \mathsf{TP}_i  =  \sum_{b_i \in C_{(\setminus j)}} \mathsf{TP}_i $ and $ \mathsf{TP}_j - \mathsf{FP}_j < 0 $, then 
		\[
		\mathsf{UB}(\mathsf{TP}_{C}-\mathsf{FP}_{C}) < \mathsf{UB}(\mathsf{TP}_{C_{(\setminus j)}}-\mathsf{FP}_{C_{(\setminus j)}})
		\]
	\end{proof}

	\begin{remark}
		In the MaxSAT Query, feature $ j $ can be eliminated in two ways: (i) removing the column associated with feature $ j $ from the  training set and (ii)  adding a hard clause $ S_j^i:= \neg b_j^i , \forall i$ with weight $ \mathsf{wt}(S_j^i)=\infty $. 
	\end{remark}

\section{Iterative Clause Learning}
\label{sec:iterative_learning}
	
	We design an iterative clause learning technique motivated by the set covering algorithm, also known as  the separate-and-conquer algorithm in symbolic rule learning~\cite{furnkranz1999separate}.
	A separate-and-conquer algorithm searches for a clause that explains/covers a part of the training set, separates samples covered by the clause, and recursively conquers the samples by learning more clauses until no samples remain. A family of rule learning approaches share the same top-level outer loop of the separate-and-conquer algorithm.
	The major difference among all approaches  is how they learn individual clauses, and in this paper we learn individual clauses using the MaxSAT-based formulation. We organize this section as follows. We first discuss which samples to  eliminate in Section~\ref{sec:sample_elimination}, formulate the objective function for the iterative approach in Section~\ref{sec:obj_iterative}, discuss the MaxSAT encoding in Section~\ref{sec:encoding_iterative} and  the early terminating condition of the iterative approach in Section~\ref{sec:termination_iterative}. 
	
	\subsection{Sample Elimination}
	\label{sec:sample_elimination}
	In the MaxSAT formulation in Section~\ref{sec:encoding}, the number of clauses in the query is linear with the number of clauses $ k $ in the desired rule $ \Rule $. We can improve this formulation by learning one clause at a time for at most $ k $ times and then merge all clauses using Boolean conjunction. Since the learned rule is in conjunction with each other, at each iteration we remove samples that are predicted false by the learned clause. In the following, we show that the removed samples are also predicted false by $ \Rule $.

	\begin{theorem}
		\label{theorem:sample_remove}
		In the iterative clause learning approach, let $ \Rule $ be the learned rule and  $ \clause(\Rule,t) $ be the learned clause at the $ t $-th iteration. Let $ \mathbf{x}  $ be the vector of  Boolean features of a sample and  $ \mathbf{x} $ is predicted false by $ \clause(\Rule,t) $, i.e., $ \bigvee_{j:b_j^t \in \clause(\Rule,t)} x_j=0 $.
		Then the prediction of $ \mathbf{x} $ by the rule  $ \R $ is false, i.e, $ \Rule(\mathbf{x}) = 0 $. 
	\end{theorem}
	\begin{proof}
		\red{rewrite}
		According to the the construction of a $ k $-clause CNF rule $ \Rule $, 
		
		\[
			\Rule(\mathbf{x})=\bigwedge_{i=1}^k \bigvee_{j:b_j^i \in \clause(\Rule,i)} x_j 
		\]
		\[
		\hat{y}(\mathbf{x})= \bigwedge_{i=1}^k \bigvee_{j=1}^m x_jw_{i,j}
		\]  
		
		Since $ (\bigvee_{j:b_j^t \in \clause(\Rule,t)} x_j)=0 $, we reach the following conclusion. 
		\[
		\begin{split}
		\Rule(\mathbf{x})&= \bigwedge_{i=1}^k \bigvee_{j:b_j^i \in \clause(\Rule,i)} x_j \\
		&=\bigvee_{j:b_j^t \in \clause(\Rule,t)} x_j \wedge  \bigwedge_{i=1, i \ne t }^k \bigvee_{j:b_j^i \in \clause(\Rule,i)} x_j \\
		&= 0 \wedge \bigwedge_{i=1, i \ne t }^k \bigvee_{j:b_j^i \in \clause(\Rule,i)} x_j\\
		&=0
		\end{split}
		\] 
		%			\[
%			\hat{y}(\mathbf{x})= \bigwedge_{i=1}^k \bigvee_{j=1}^m x_jw_{i,j}=(\bigvee_{j=1}^m x_jw_{r,j}) \wedge  \bigwedge_{i=1, i \ne r }^k \bigvee_{j=1}^m x_jw_{i,j}= 0 \wedge \bigwedge_{i=1, i \ne r }^k \bigvee_{j=1}^m x_jw_{i,j}=0
%			\] 
			\end{proof}

	\subsection{Objective Function}
	\label{sec:obj_iterative}
	 We now  define the objective function in the iterative approach. The major difference  in the objective function with Eq.~\ref{eq:obj} is that  the number of samples differs  in each iteration as we eliminate  a subset of samples that are predicted false by the learned clause. Let $ k $ be the number of clauses in the desired rule and clause $ \clause(\Rule,t) $ be learned  at the $ t $-th iteration.	Given a training set $ (\mathbf{X}, \mathbf{y})$ of size $ n $ with each sample having $ m $ binary features, let $ n_t $ be the size of the training set  at the $ t $-th iteration, where $ t=1, \dots, k $ and $ n_1=n $. Let $\mathcal{E}_{\clause(\Rule,t)} $ be the set of samples that are  predicted incorrectly by $ \clause(\Rule,t) $, i.e., $ \mathcal{E}_{\clause(\Rule,t)} = \{(\mathbf{X}_i,y_i) | y_i \oplus \bigvee_{j:b_j^t \in \clause(\Rule,t)} \mathbf{X}_{i,j}= 1 \} $.	Given the data-fidelity parameter $ \lambda $,  we optimize the following function at the $ t $-th iteration. 
	
	\begin{equation}
	\label{eq:obj_iterative}
	\min_{{\clause(\Rule,t)}} \quad \frac{\lambda}{n} \sum_{i=1}^{n_t}|\mathcal{E}_{\clause(\Rule,t)}| + \frac{(1-\frac{n_t}{n}\lambda)}{mk}|{\clause(\Rule,t)}|
	\end{equation}

	The objective function in Eq.~\ref{eq:obj_iterative} ensures that the penalty on prediction error of a sample is  same in all iterations, which is $ \frac{\lambda}{n} $.  Since we emphasis the objective-value  to be $ 1 $ in the worst case as in Eq.~\ref{eq:obj},  the penalty on selecting a feature in the $ t $-th clause is set to $ \frac{(1-\frac{n_t}{n}\lambda)}{mk} $. As a  subset of training set is removed at each iteration ($ n_t \ge n_{t+1} $), the penalty on rule-sparsity monotonically increases as the iteration advances. As a result, the objective function prefers smaller clauses as we progress in the iterative approach. 
	
	\subsection{MaxSAT Encoding}
	\label{sec:encoding_iterative} 
	To learn clauses in the iterative approach, the MaxSAT query presented in Section~\ref{sec:encoding} has to be modified. The soft clauses $ E_q $ and $ S_j^i $ are kept same as in Eq.~\ref{soft_clause_error} and~\ref{soft_clause_feature} respectively while their weights are modified based on the co-efficients of prediction error and rule-sparsity in the objective function in Eq.~\ref{eq:obj_iterative}.  In particular, we set $ \mathsf{wt}(E_q)=\frac{\lambda}{n} $ and $ \mathsf{wt}(S^i_j)=\frac{(1-\frac{n_t}{n}\lambda)}{mk} $. Finally, we construct the hard clause $ H_q $ by setting $ k=1 $ in Eq.~\ref{hard_clause_rule_consistency} as we  learn one clause at each iteration. 
	
	\subsection{Terminating Condition:}
	\label{sec:termination_iterative}
	As our goal is to learn a $ k $-clause rule $ \Rule $, the presented iterative approach is repeated for at most $ k $ iterations. However, it is possible to terminate early if  $ \clause(\Rule, t) $ can not cover any new sample in the training set at the $ t $-th iteration. In that case, $ \clause(\Rule, t) $ is not included in $ \Rule $ and the iterative process terminates. We summarize our discussion in the following theorem.

	\begin{theorem}
		\label{thm:iterative_termination}
		Let $ (\mathbf{X}, \mathbf{y}) $ be the training set and $ \clause(\Rule,t) $ be the learned clause at the $ t $-th iteration. If  all samples in $ (\mathbf{X}, \mathbf{y}) $ are predicted true (i.e, 1)  by $ \clause(\Rule,t) $, that is, $ \bigvee_{j:b_j^t \in \clause(\Rule,t)} \mathbf{X}_{i,j} =1, \forall i$, then $ \clause(\Rule,t) $ is not included in $ \Rule $ and the iterative approach terminates after iteration $ t $. 
	\end{theorem}
			
%	\begin{theorem}
%		Suppose clause $ \mathbf{w}_r $ is learned at the $ r $-th iteration. If $ \sum_{i=1}^{n_r} \mathds{1}_{\bigvee_{j=1}^mx_{i,j}w_{r,j}=0}=0 $, then $  \mathsf{w}_r $ is not included in classifier $ \hat{y} $ and the iterative process terminates.  
%	\end{theorem}
	
	\begin{proof}
		\red{rewrite}
		 According to Theorem~\ref{theorem:sample_remove}, $ (\mathbf{X}, \mathbf{y}) $ consists of samples that are predicted true by $ \clause(\Rule,t-1) $  learned at iteration $ t-1 $.  Since $ \forall i,  (\bigvee_{j:b_j^t \in \clause(\Rule,t)} \mathbf{X}_{i,j}) =1 $, $ \clause(\Rule,t) $ only covers ( i.e., predicts true) a sample that is also covered by $ \clause(\Rule,t-1) $. Therefore, $ \clause(\Rule, t) $ is redundant  and hence not included in $ \Rule $.

%		 Since $ \sum_{i=1}^{n_r} \mathds{1}_{\bigvee_{j=1}^mx_{i,j}w_{r,j}=0}=0 $,  all training samples are  predicted \emph{true} by $ \mathbf{w}_r $ and no sample is predicted \emph{false}. Therefore, all samples at iteration $ r $ is covered by $ \mathbf{w}_{r-1} $, hence $ \mathbf{w}_r $ is not included in the classifier rule.   
		
		Since $ \clause(\Rule, t) $ predicts all samples as true, $ (\mathbf{X}, \mathbf{y}) $ will also be the training set at iteration $ t+1 $ because no sample is removed (Theorem~\ref{theorem:sample_remove}). Therefore, the iterative approach will learn the same clause again, hence the approach can be terminated

\end{proof}

	\begin{algorithm}
		\caption{Iterative  clause learning}
		\begin{algorithmic}[1]
			\Function{\iterativeClauseLearning}{$ \mathbf{X},\mathbf{y}  ,k,\lambda $}
			\State $ \Rule=\{\} $
			\For{$ t=1, \dots, k $} \label{alg:itr_for_start}
			\State $ Q,W\leftarrow \maxsatquery(\mathbf{X},\mathbf{y},\lambda) $ \label{alg:itr_constructQuery}
			\State $ \sigma^* \leftarrow \MaxSAT(Q,W) $  \label{alg:itr_MaxSATSolving}
			\State $ C \leftarrow \createclause(\sigma^*) $
			\label{alg:itr_createClause}
			\If{$ \bigvee_{j:b_j^t \in C} \mathbf{X}_{i,j} =1, \forall i$} \label{alg:itr_termination_check}
			\State break \label{alg:itr_terminate}
			\EndIf
			\State $\clause(\Rule, t)\leftarrow C $ \label{alg:itr_clauseAdd}
			\State $ (\mathbf{X},\mathbf{y}) =\{(\mathbf{x},y) \in (\mathbf{X},\mathbf{y})| \bigvee_{j:b_j^t \in \clause(\Rule,t)} \mathbf{x}_{j} = 1 \}  $ \label{alg:itr_removeSamples}
			\EndFor 
			\Return $ \Rule $ \label{alg:itr_for_end}
			\EndFunction
		\end{algorithmic}
	\label{alg:iterative}
	\end{algorithm} 

\subsection{Description of Algorithm}
We show the algorithm for iterative clause learning in Algorithm~\ref{alg:iterative}. The algorithm takes  in inputs as  the training dataset $ (\mathbf{X}, \mathbf{y}) $, the data-fidelity parameter $ \lambda $, and the number of clauses $ k $ in the desired rule   and outputs the learned rule  $ \Rule $. Initially $ \Rule $ is an empty rule. The main loop in the algorithm repeats for at most $ k $ times while learning one clause in each iteration (Line~\ref{alg:itr_for_start}--\ref{alg:itr_for_end}). Inside the loop, the function {\maxsatquery}  in Line~\ref{alg:itr_constructQuery}  constructs the MaxSAT query $ Q $ and the weight $ W $ of clauses in $ Q $ for the dataset $ (\mathbf{X}, \mathbf{y}) $ as described in Section~\ref{sec:encoding_iterative}. A MaxSAT solver takes in $ Q $ and $ W $ as inputs, solves the query and returns the optimal assignment $ \sigma^* $ (Line~\ref{alg:itr_MaxSATSolving}). Based on the assignment, function {\createclause} in Line~\ref{alg:itr_createClause} constructs a clause $ C $ as described in Construction~\ref{construction:rule}. Then the algorithm checks if the learned clause $ C $ can cover any new sample in the training set in Line~\ref{alg:itr_termination_check}. If  $ C $ does not cover any new sample, $ C $ is not added in Rule $ \Rule $ and the learning process terminates according to Theorem~\ref{thm:iterative_termination} (Line~\ref{alg:itr_terminate}), otherwise $ C $ is added in $ \Rule $ (Line~\ref{alg:itr_clauseAdd}). Finally, a subset of samples that are predicted false are removed from the training dataset (Line~\ref{alg:itr_removeSamples}) and then process repeats.

\section{Incremental Mini-batch Rule Learning}
\label{sec:incremental_learning}
In this section, we propose a mini-batch rule learning approach that learns the  classification rule $ \Rule $ incrementally over batches.  
Since the complexity of  the MaxSAT encoding in Section~\ref{sec:encoding} depends on the size of the training set, we propose a mini-batch learning framework to reduce the number of clauses in the MaxSAT query with the aim of reducing the solution time of the query. In this approach, we select a smaller-size batch randomly from the full training set, learn a rule on the batch such that we can minimize the change in the learned rule compared to the  rule  in the previous batch while maximizing the prediction accuracy in the current batch. We repeat this process for a fixed number of iterations to learn a stable rule.   In the following, we discuss the objective function in Section~\ref{sec:obj_incremental} and then discuss the MaxSAT encoding in Section~\ref{sec:encoding_incremental}.

\subsection{Objective Function:}
\label{sec:obj_incremental}
In the incremental mini-batch learning, we design an objective function to penalize both the prediction error and the change of selection of features in the rule across consecutive batches. Let $ \tau $ be the number of iterations of the learning process and $ (\mathbf{X}',\mathbf{y}') $ be the set of  randomly chosen  samples from the training set $ (\mathbf{X},\mathbf{y}) $ of size $ n $.  We also consider $ \Rule_t $ being the $ k $-clause learned rule in the $ t $-th iteration ($ t=1, \dots, \tau $), where $ \Rule_0 $ is an empty rule. To measure the prediction error on the current batch, we consider $ \mathcal{E}_{\Rule_t} =\{(\mathbf{x},y) \in (\mathbf{X}',\mathbf{y}') | y \ne \Rule_t(\mathbf{x}) \} $ as  the set of misclassified samples from  $ (\mathbf{X}',\mathbf{y}') $. In addition, we encode the change in the rules learned in two consecutive iterations in terms of the difference of the rule-size $ |\Rule_t| - |\Rule_{t-1}| $. Given the data-fidelity parameter $ \lambda \in [0,1] $ and learning rate $ \alpha \in \mathcal{R}^+ $,  we optimize the following function at each iteration of the mini-batch setting.

%The objective function in Eq.~\ref{eq:obj}  considers both prediction accuracy and sparsity of rules while finding the optimal assignment of noise variables and feature variables. Unlike optimizing rule-sparsity  in Eq.~\ref{eq:obj}, the new objective function for incremental approach  penalizes the different assignment of a feature variable compared against its assignment in the previous epoch. Moreover, the weight on this penalty increases gradually so that the alteration  in the assignment of a feature variable is less preferred in later epochs.  

\begin{equation}
	\label{eq:obj_incr}
	\min_{\Rule_t} \quad \frac{\lambda^{1+\frac{t-1}{\alpha (\tau-1)}}}{n} |\mathcal{E}_{\Rule_t}|+\frac{1-\lambda^{1+\frac{t-1}{\alpha (\tau-1)}}}{m k} (|\Rule_t|-|\Rule_{t-1}|)
\end{equation}

\red{$ \Delta=1-\lambda \text{ if  } \alpha \ge 0 \text{, otherwise }  \Delta=\lambda $}

\red{$\lambda$=$\lambda + \alpha \Delta \frac{t-1}{T}$, $ \alpha \in [-1,1] $}

\red{redefined}
\begin{equation}
\label{eq:obj_incr}
\min_{\Rule_t} \quad \frac{\lambda + \alpha \Delta \frac{t-1}{T}}{n} |\mathcal{E}_{\Rule_t}|+\frac{1-(\lambda + \alpha \Delta \frac{t-1}{T})}{m k} (|\Rule_t|-|\Rule_{t-1}|)
\end{equation}

In the objective function, the data-fidelity parameter $ \lambda $ has an exponent $ 1+\frac{t-1}{\alpha (\tau-1)} \in [1, 1+ \frac{1}{\alpha}] $. Since $ \lambda \in [0,1] $ and $ \alpha \in \mathcal{R}^+ $, this exponent decides  how much $ \lambda $ will decrease from its initial value as the iteration $ t $ progresses. Here $ \alpha $ decides the amount of decrease of $ \lambda $ from its initial value and acts as an inverse to the stability of the rule.  Moreover, as iteration $ t $ progresses,  the objective function tries to learn a more stable rule by putting a less penalty on the prediction error. 
In this context, the penalty on the prediction error also depends on the size of the batch since we apply the size $ n $ of the full training set to normalize the penalty on  prediction error. Intuitively, if the batch-size is close to the size of the training set, more priority is given to the prediction accuracy  and vice versa.

\subsection{MaxSAT Encoding of Mini-batch Learning}
\label{sec:encoding_incremental}
We now discuss the MaxSAT encoding for the incremental mini-batch learning. The soft clause $ E_q $ associated with noise variables is identical to  Eq.~\ref{soft_clause_error} and the weight of this soft clause is set to $\frac{\lambda^{1+\frac{t-1}{\alpha (\tau-1)}}}{n}$.  The hard clause $ H_i $ is  identical to Eq.~\ref{hard_clause_rule_consistency} because at each iteration, we learn a $ k $-clause rule. Finally, soft clause $ S_j^i $ is modified according to the objective function as follows: 

\[
S_j^i:=
\begin{cases}
b_j^i& \text{if }  x_j \in  \clause(\Rule_{t-1},i)  \\
\neg b_j^i & \text{otherwise}
\end{cases};\qquad \mathsf{wt}(S_j^i)=\frac{1-\lambda^{1+\frac{t-1}{\alpha (\tau-1)}}}{m k}
\]

In the definition of $ S^i_j $, a feature variable $ b^i_j $ is preferred to keep its assignment in the previous iteration, otherwise the objective function is incurred a cost $ (1-\lambda^{1+\frac{t-1}{\alpha (\tau-1)}})/m k $. Intuitively,  in the optimal solution at iteration $ t $, if each feature variable is assigned to its previous assignment,  the hamming distance between two consecutive rules is zero.

%Initially each $ w_{r,j} = 0 $, hence $ S_{r,j}:= \neg w_{r,j} $ in the $ 1^\text{st} $ epoch. 

\subsection{Iterative Clause Learning in Mini-batch Setting}

We now discuss a more improved learning framework by merging both iterative clause learning approach and incremental mini-batch learning approach with an  incorporation of  feature-ranking.   In this framework, we consider a percentage of higher ranked features as described in Section~\ref{sec:feature_elimination}. Then we iteratively learn clauses on a reduced set of features, where each clause is learned in an incremental mini-batch setting. 

\label{sec:all_hypotheses}
\[
\min_{w_{r,j}} \quad \frac{\lambda^{f(t)}}{n^{(t)}} \sum_{i=1}^{n^{(t)}}\eta_i+\frac{(1-(\frac{n_i}{n}\lambda)^{f(t)})}{m k} \sum_{r=1}^k\sum_{j=1}^{m} {w^{(t)}_{r,j}- w^{(t-1)}_{r,j}} 
\]
\[
f(t)=\frac{t-1}{Tc}
\]

\red{redefined}
\[
\min_{w_{r,j}} \quad \frac{\lambda + \alpha \Delta \frac{t-1}{T}}{n^{(t)}} \sum_{i=1}^{n^{(t)}}\eta_i+\frac{(1-\frac{n_i}{n}(\lambda + \alpha \Delta \frac{t-1}{T}))}{m k} \sum_{r=1}^k\sum_{j=1}^{m} {w^{(t)}_{r,j}- w^{(t-1)}_{r,j}} 
\]

\section{More Constraints on Desired Rule:}

For the sake of interpretability, we can put additional constraints to control the rule-size and  also the preference  of an individual feature in the desired rule. For example, maximum clause-size constrains the maximum number of selected features in a clause. Let assume that, $ \sigma_i \in \{1,\dots,m\} $ is an integer  number that denotes the maximum number of selected features that the $ r $-th clause can have.\footnote{In our formulation, it is straightforward to have different  $ \sigma_i $ for different clauses.} 
\[
\sum_{j=1}^m b_j^i \le \sigma_i
\]
The above constraint is a pseudo-boolean constraint and can be encoded into CNF using an off the shelf pseudo-boolean to CNF encoder (i.e., PBEncoder~\cite{philipp2015pblib}). After encoding, we put $ \infty $ weight to each clause in the encoded CNF and append in the MaxSAT query $ Q $ as hard clauses. 

We also constrain the maximum number of selection of an individual feature in the desired rule by introducing an integer threshold $ \theta_j $ corresponding to the $ j $-th feature. 
\[
\sum_{i=1}^k b_j^i \le \theta_j
\]  
The above constraint is similarly encoded to CNF and then added to $ Q $ has hard clauses. For protected features such as age, ethnicity, sex etc., we can set corresponding $ \theta_j=0 $ so that the desired rule does not include these features in the classification rule.
