# Supplementary material for: Efficient Learning of Interpretable Classification Rules
Source: arXiv:2205.06936 source file (2022-08-30)
Supplement: Supplementary file 3 [file incMLIC.tex]

\section{ {\Framework}: }\label{sec:framework} 
\textcolor{red}{Change weight of each soft clause\\}
In this section, we present the primary contribution of this paper, {{\Framework}}, which is a MaxSAT-based incremental learning framework for interpretable classification rules. The core technical idea behind {{\Framework}} is to divide the training data into a fixed number $ p $ of partitions {and employ {\MaxSAT} based learning framework for each partition } such that the MaxSAT query constructed for partition $i$ is based on the training data for partition $i$ and the rule learned until partition $i-1$.
 To this end, we use the notation $(\mathbf{X}^i, \mathbf{y}^i) $ to refer to the training data for the $i$-th partition. We assume that  $\forall i, |\mathbf{X}^i| = |\mathbf{X}^{i-1}|$.

%The rest of the section is organized as follows: we first describe the construction of {MaxSAT} query for the  $i$-th partition  in Sect.~\ref{subsec:query} to learn CNF rules, and then discuss the discretization techniques for real-world datasets in Sect.~\ref{sec:nonbinaryfeatures}. The incrementality of {{\Framework}} gives rise to the challenge of having redundant literals in the learned rules; we address such redundancy in Sect.~\ref{sec:pruning} and finally we discuss, in Sect.~\ref{sec:dnf}, how our framework for learning CNF rules can be easily extended to learn DNF rules as well.  We provide an illustration of rule learning of {\Framework} in Appendix ~\ref{sec:example}. 

	\subsection{Construction of MaxSAT Query}\label{subsec:query}

  We now discuss the construction of a  {MaxSAT} query, denoted by $Q_i$, for the  $i$-th partition ($i \in [1,p]$). To construct the {MaxSAT} query for the $i$-th partition, we assume an access to the rule learned from the  $(i-1)$-th partition (where $\R_0$ is  an empty formula). 
  
 The construction of $Q_i$ takes in four parameters: (i) $ k $, the desired number of clauses in CNF rule, (ii) $ \lambda $, the data fidelity parameter, (iii) a matrix ${\mathbf{X}^{i}} \in \{0,1\}^{n \times m}$  describing the  binary value of  $m$ features for each of    $n$ samples with $\mathbf{X}^{i}_q$ being a binary valued vector for the $ q $-th sample corresponding to feature vector $\mathbf{x} = \{x_1, x_2, \dots, x_m\}$, (iv) a label vector $\mathbf{y}^{i} \in \{0,1\}^n$ containing a class label $y^{i}_q$ for the  sample $\X^{i}_q$.   Consequently, {{\Framework}} constructs a {MaxSAT} query for the $ i $-th partition and invokes an off-the-shelf MaxSAT solver to compute the underlying rule $ \R_i $.

	{\Framework} considers two types of propositional variables: (i) feature variables and (ii) noise (classification error) variables.
%	 Feature variables are defined once for all partitiones. 
 	For the $ i $-th partition, {\Framework} formulates a classifier rule $ \R_i $ based on following intuition.  Recall, a $ k $-clause CNF rule $ \R_i=\bigwedge_{l=1}^kC_l $ is  represented as the conjunction of  $ k $ clauses where clause $ C_l $ is the disjunction of  feature variables. A  sample $ \X^i_q $ satisfies  $ C_l $ if $ \X^i_q $ has at least one similar feature whose representative variable is present in $ C_l $. If $ \X^i_q $ satisfies  $ \forall l, C_l$, then  $ \R_i(\X^i_q)=1 $ otherwise $ \R_i(\X^i_q)=0 $. Since  feature $ x_j $ can be present or not present  in each of   $ k $ clauses, {\Framework} considers $ k $  boolean variables, each denoted by $ b_j^l $ ($ l \in [1,k] $) for  feature $ x_j $ to denote its participation in the $ l $-th clause. A sample $ \X^i_q $, however, can be misclassified by $ \R_i $ i.e., $ \R_i(\X^i_q)\oplus  y_q^i =1 $.  {\Framework}  introduces  a noise variable $ \eta_q $ corresponding to  sample $ \X^i_q $ so that the assignment of $ \eta_q $ can be interpreted whether $ \X^i_q $ is misclassified by $ \R_i $ or not.  Hence the key idea of {{\Framework}} for learning the $ i $-th partition is to define a {MaxSAT} query over $k \times m + n$ propositional variables, denoted by $\{ b_{1}^{1}, b_{2}^{1}, \dots ,b_{m}^{1}, \dots ,b_{m}^{k}, \eta_1, \dots ,\eta_n\}$.   The {\MaxSAT} query of {\Framework} consists of the following three sets of constraints:

	\begin{enumerate}
		
		\item Since our objective is to find sparser rules, the default objective of  {\Framework} would be to add a constraint to falsify as many $ b_j^l $  as possible. 	As noted earlier,  rule $\Rule_{i-1}$ from the $(i-1)$-th partition plays an important role in the construction of MaxSAT 
		constraints of the $i$-th partition. Therefore,   if $x_{j} \in \clause(R_{i-1},l)$, {\Framework} would deviate from its default behavior by adding a constraint to keep the corresponding literal $ true $ in the optimal assignment.  The weight corresponding to this clause is $ 1 $. We formalize our discussion as follows:
	\begin{equation*}
	V^l_j:= 
	\begin{cases}
	b^l_j&\quad \text{if }  x_{j} \in \clause(\R_{i-1},l)\\
	\neg b^l_j&\quad \text{otherwise } \\
	\end{cases}
	;\quad  W(V^l_j)= 1
	\label{eq:constraint-v}
	\end{equation*}
		\item We use noise variables to handle mis-classifications and therefore, {\Framework} tries to falsify as many   noise variables as possible. Since data fidelity parameter $ \lambda $ is proportionate to accuracy, {\Framework} puts $ \lambda $ weight to each following soft  clause. 

		\begin{equation*}
		N_q:= (\neg \eta_q ); \qquad \qquad W(N_q) = \lambda
		\label{eq:constraint_two}
		\end{equation*}
		%		Here $N_i $ is also a soft clause. 
		
		\item 
		Let $\mathbf{B}_{l} = \{b^{l}_{j} \mid j \in [1,m] \}$. 
		Here we provide the third set of constraints of {\Framework}. 
		\begin{equation*}
		D_q:= (\neg \eta_q \rightarrow ( y_q \leftrightarrow \bigwedge_{l=1}^{k} ({\mathbf{X}_q} \vee {\mathbf{B}_{l}})));    W(D_q) = \infty
		\label{eq:constraint_three}	
		\end{equation*}
		Every hard clause $D_q$  can be interpreted as follows. If $\eta_q$ is assigned to \textit{false} ($ \neg \eta_q = true$) then ${y}^i_q = \R_i(\X^i_q)=\bigwedge_{l=1}^{k} ({\mathbf{X}_q} \vee {\mathbf{B}_{l}})$.  The operator ``$\vee  $'' is defined in Sect. \ref{sec:preliminaries}.  
		
		%		We are not showing in details how $ D_i $ can be encoded into CNF forms using standard procedure. We refer \cite{MM18} for detailed description.

	\end{enumerate}
	Finally, the set of constraints $Q_i$ for  the $ i $-th partition constructed by {{\Framework}} is defined as follows:
	\begin{equation*}
	\label{eq:constraint-imli}
	Q_i :=  \bigwedge_{j=1, l = 1}^{j=m,l=k} V^l_j \wedge \bigwedge_{q=1}^{n} N_q \wedge \bigwedge_{q=1}^{n} D_q
	\end{equation*} 
	
	Next, we extract $\Rule_i$ from the solution of $Q_i$ as follows. 
	\begin{construction}
		Let $\sigma^* = \MaxSAT(Q_i,W)$, then $x_j \in {\clause(\Rule_i,l)}$ iff $\sigma^*(b_{j}^{l}) = 1$.
	\end{construction}
	In the rest of the manuscript, we will use $\Rule$ to denote $\Rule_{p}$.  
	\subsection{Beyond Binary Features}\label{sec:nonbinaryfeatures}

	We have considered that the feature value of a training sample is binary. Real-world  datasets, however,  contain categorical, real-valued or numerical features. We use the standard discretization technique to convert categorical and continuous (real or integer value) features to boolean features. We use  {\em one hot encoding} to convert categorical features to binary features by introducing a boolean vector  with the cardinality equal to the number of distinct categories of individual categorical features.
	\begin{example}
		\label{ex:bin_categorical}
		Consider a categorical feature with three categories: ``red'', ``green'', ``'yellow''. One hot encoding would convert this feature to three binary variables, which take values $ 100 $, $ 010 $, and $ 001 $ for the three categories.
	\end{example}
	
	 Furthermore, we can discretize the continuous-valued features into  binary features by comparing the feature value to  a collection of  thresholds within range and introducing  a boolean feature vector with cardinality proportional to the number of considered threshold.
Specifically, for a continuous feature $ x_c $ we consider a number of thresholds $ \{\tau_1,\dots,\tau_t\}$ where $  \tau_i < \tau_{i+1}  $ and define two separate Boolean features $ I[x_c \ge \tau_i] $ and $ I[x_c < \tau_i] $ for each $ \tau_i $. 
	We present the following definitions based on the discretization of  continuous features.
	
		 	\begin{definition}
		 		$ tval(b): b \rightarrow \tau $ is a function over boolean variables corresponding to discretized binary features (from a continuous feature) and outputs the compared threshold value. 
		 	\end{definition}
		 	
		 	\begin{definition}
		 		$ op(b): b \rightarrow \{\ge , <\} $ is a function over boolean variables corresponding to discretized binary features (from a continuous feature) and outputs the comparison operator between continuous feature value and $ tval(b) $. 
		 	\end{definition}
		 	
		 	\begin{definition}
		 		$ siblings(b_i, b_j): (b_i, b_j) \rightarrow \{true, false\} $ is a function over pair of  boolean variables $ b_i,b_j $ and outputs $ true $ if the boolean features corresponding to $ b_i,b_j $ are constructed by discretizing the same continuous feature  
		 		and  
		 		$ op(b_i)=op(b_j) $.
		 	\end{definition}
	 	
%	 	\begin{example}
%	 		\label{ex:bin_categorical}
%	 		Consider a categorical feature with three categories: ``red'', ``green'', ``'yellow''. One hot encoding would convert this feature to three binary variables, which take values $ 100 $, $ 010 $, and $ 001 $ for the three categories.
%	 	\end{example}
	 	\begin{example}
	 		\label{ex:bin-continuous}
	 		Consider  a  continuous feature $ x_c $ with range $  (0,100) $ and three thresholds $ \{25,50,75\} $ associated with this feature.  $ \Framework $ introduces $ 6 $ new boolean features   $ \{ x_1: I[x_c\ge 25],x_2: I[x_c\ge 50], x_3:I[x_c\ge 75], x_4:I[x_c< 25], x_5:I[x_c< 50],x_6:I[x_c < 75]\} $. Following this discretization technique,  the binary feature vector  of a sample  with   feature value $ x_c=37.5 $ is  $ 100011 $, because among the $6  $ introduced boolean features $ x_1:I[ 37.5 \ge 25 ]=1$, $ x_5:I[37.5 < 50]=1 $, and $x_6:I[ 37.5 < 75]=1 $.

	 	\end{example}
	 	
	 	\begin{example}
	 		\label{ex:prune}
	 		In Example \ref{ex:bin-continuous}, $ b_i $ is a boolean variable corresponding to feature $ x_i $. Now $ tval(b_1)=25$, $ op(b_1)=\text{``}\ge\text{''}$, $ siblings(b_1,b_2)=true, $ and $ siblings(b_1,b_4)=false $. 
	 	\end{example}

	\subsection{Redundancy Removal}\label{sec:pruning}
	Given the incremental procedure of learning {\Rule} where the constraints for the $i$-th partition are influenced from the rule learned until the $(i-1)$-th partition, one key challenge is to address potential redundancy in the learned rules. In particular, we observe that redundancy manifests itself in binary features corresponding to continuous-valued features as the $(i-1)$-th partition  might suggest inclusion of feature  $ I[x_c < \tau_u] $ while the $ i $-th partition  also suggests inclusion of feature $ I[x_c < \tau_v] $ where $\tau_u \ne \tau_v$. To this end, we present Algorithm \ref{alg:imli-RRL} to remove redundant literals. 

	\begin{algorithm}
		\caption{Remove Redundancy}\label{alg:imli-RRL}
		\begin{algorithmic}[1]
			\Procedure{removeRedundantLiterals}{$\R$}
			\For{each  clause $ C_l $ of $ \R $} 
			\For{ each pair $ \langle b_i^l,b_j^l \rangle $  where   $ \sigma(b_i^l)=\sigma(b_j^l)=1$,   $siblings(b_i^l,b_j^l)=true $, and $ tval(b_i^l) < tval(b_j^l) $ }
			\If {$op(b_i^l)=op(b_j^l)=\text{``}\ge \text{''} $}
			\State  $ \R'=\R[\sigma(b_j^l)\mapsto0] $ \Comment{$ b_j^l $ is redundant}
			\Else \State $ \R'=\R[\sigma(b_i^l)\mapsto0] $
			\EndIf
			\EndFor
			\EndFor
			\State \Return $ \R' $
			\EndProcedure
		\end{algorithmic}
	\end{algorithm}

	\begin{lemma}
		 $ |\R'| \le |\R| $ and $ \R' $ is equivalent to $ \R $. 
		
		\label{lm:adjustment_of_rule_size}
	\end{lemma}
\begin{proof}
	\label{prf:prune}
	%		Removed due to the brevity of presentation.
	The case  $ |\R'|=|R| $ is trivial because no literal is removed from $ \R' $, and $ \R' $ is equivalent to  $ \R $.

	When $ |\R'| < |\R| $, $ \exists \langle b_i^l,b_j^l \rangle $  where $  l \in [1,k] $,    $siblings(b_i^l,b_j^l)=true $, $ tval(b_i^l) < tval(b_j^l) $, and $ x_c $ is the considered continuous feature. 
	
	Suppose  $op(b_i^l)=op(b_j^l)=\text{``}\ge \text{''} $. Consider two sets of real number: $ S_i= \{x_i: x_i \ge  tval(b_i^l)\} $ and $ S_j=\{x_j: x_j \ge  tval(b_j^l)\} $. As $ \R $ is in CNF,  $ \R $ checks $ I[x_c \in S_i \cup S_j] $  to classify  $ \forall q,\mathbf{X}_q  $. Here $ S_i \cup S_j = S_i $, so $ b_j^l $ can be pruned.
	
	We can prove similarly when $op(b_i^l)=op(b_j^l)=\text{``}< \text{''} $.
	
	Therefore, $ |\R'| \le |\R| $ and $ \R' $ is equivalent to $ \R $.
	
\end{proof}

	\subsection{Learning DNF Rules}
	\label{sec:dnf}

			Primarily we focus on learning rule $ \R $ which is in CNF form. We can also apply incremental technique for learning DNF rules.   Suppose, we want to learn a rule $ y=S(x) $ where $ S(x) $ is expressible in DNF. We show that $ y = S(x) \leftrightarrow \neg (y=\neg S(x)) $. Here $ \neg S(x) $ is in CNF.  Therefore, to learn DNF rule $ S(x) $, we simply call {\Framework} with $ \neg \mathbf{y} $ as input  for all $ p $ batches, learn CNF rule, and finally
	negate the learned rule.  Hence Algorithm \ref{alg:imli-RRL} can be directly applied.
	\begin{example}
		\label{ex:dnf_rule}
		``$( \text{is Male}\vee \text{Age}<\text{50})\wedge(\text{Education}=\text{Graduate}\vee\text{Income}\ge\text{1500}) $''\textemdash rule is  learned for negated class label. The resultant DNF rule is  ``$ (\text{is not Male}\wedge  \text{Age}\ge\text{50}) \vee (\text{Education} \ne \text{Graduate}\wedge\text{Income}<\text{1500} )$'' 
	\end{example}
