# Supplementary material for: Efficient Learning of Interpretable Classification Rules
Source: arXiv:2205.06936 source file (2022-08-30)
Supplement: Supplementary file 4 [file proposed_improvement.tex]

\section{Convert to MDP}
	
	\textcolor{red}{change $ \tau $ in previous section}

	Markov decision process is a $ 4 $-tuple $ (S,A,P_a,R_a) $ where 
	
	\begin{itemize}
		\item $ S $ is a finite set of states.
		\item $ A $ is a finite set of actions (alternately, $ A_s $ is the finite set of actions available from state $ s $).
		\item $ P_a(s,s')=\probability(s_{i+1}=s' | s_i=s, a_i=a) $ is the probability that action $ a $ in state $ s $ at time $ i $ will lead to state $ s' $ at time $ i+1 $. 
		\item $ R_a(s,s') $ is the immediate reward (or expected immediate reward) after transitioning from state $ s $ to $ s' $, due to action $ a $.
	\end{itemize}

	We can fit our problem as a Markov decision process as follows.
	
	\begin{itemize}
		\item We have $ \tau $ states, which is equal to the number of partitions. In state $ s_i $, we learn $ \Rule_i $. 
		\item From  each state $ s_i $, we can take two actions,  $\{ a_0,a_1 \} $ where $ a_0= \text{keep rule } \Rule_{i} $ and $  a_1 =  \text{ revert to rule } \Rule_{i-1} $
		\item  Let assume that, $ z_{i} $ is the cost function after solving the MaxSAT query $ Q_i $ in state $ s_i $. We can calculate $ z_i $ using Eq~\ref{eq:cost}.   We define transition probability as follows. 
			\[
			\begin{split}
			&P_{a_0}(s_i,s_{i+1})= \frac{1}{1+e^{z_i - z_{i-1}}}\\
			&P_{a_1}(s_i,s_{i+1})= \frac{1}{1+e^{z_{i-1} - z_i}}
			\end{split}
			\]
		Since we minimize the cost function in Eq~\ref{eq:cost}, $  P_{a_0}(s_i,s_{i+1}) > P_{a_1}(s_i,s_{i+1}) $, when $ z_i < z_{i-1} $.
		\item We define reward probability as follows. 
		\[
		\begin{split}
			&R_{a_0}(s_i,s_{i+1})=-z_i\\
			&R_{a_1}(s_i,s_{i+1})= - z_{i-1}			
		\end{split}
		\]
	\end{itemize}

%	We can consider a Markov Decision Process. In state $ S_i $, we learn rule $ R_i $. We take two actions from state $ S_i $ to $ S_{i+1} $. We can either keep rule $ R_i $, or revert to $ R_{i-1} $.  
%
%	
%	Now we have two choices: either keep rule $ \Rule_{i} $ or revert to $ \Rule_{i-1} $. We make the decision based on the value of $ z_{i} $ and $ z_{i-1} $.  We consider a probability distribution over the difference between $ z_i $ and $ z_{i-1} $ as follows. 
